# Supplementary material for: Meta-Learning to Compositionally Generalize
Source: arXiv:2106.04252 source file (2021-06-29)
Supplement: Supplementary file 1 [file appendix_subtasks.tex]

\begin{table}[ht!]
\centering
\setlength{\tabcolsep}{3pt}
\begin{tabular}{lllll}
Cogs Subtask & Baseline & Base-MAML & L-MAML & T-MAML \\
active$\rightarrow$passive  & 0.9659 & 0.9952 & 0.9405 & 0.9915 \\
cp recursion  & 0 & 0 & 0 & 0 \\
do dative$\rightarrow$pp dative  & 0.8422 & 0.8729 & 0.8469 & 0.8749 \\
obj omitted transitive$\rightarrow$transitive  & 0.7962 & 0.8705 & 0.8459 & 0.8843 \\
obj pp$\rightarrow$subj pp  & 0 & 0 & 0 & 0 \\
obj$\rightarrow$subj common  & 0.9884 & 0.993 & 0.9924 & 0.9903 \\
obj$\rightarrow$subj proper  & 0.8923 & 0.981 & 0.9847 & 0.9799 \\
only seen as transitive subj$\rightarrow$unacc subj  & 0.9415 & 0.9383 & 0.9812 & 0.9478 \\
only seen as unacc subj$\rightarrow$obj omitted transitive subj  & 0.8148 & 0.7963 & 0.8144 & 0.8115 \\
only seen as unacc subj$\rightarrow$unerg subj  & 0.8103 & 0.8047 & 0.8068 & 0.8122 \\
passive$\rightarrow$active  & 0.8814 & 0.9374 & 0.9084 & 0.8547 \\
pp dative$\rightarrow$do dative  & 0.5309 & 0.6559 & 0.6296 & 0.6769 \\
pp recursion  & 0.0003 & 0 & 0 & 0 \\
prim$\rightarrow$inf arg  & 0.2054 & 0.5214 & 0.7212 & 0.661 \\
prim$\rightarrow$obj common  & 0.3871 & 0.6163 & 0.6633 & 0.6442 \\
prim$\rightarrow$obj proper  & 0.1507 & 0.2185 & 0.2234 & 0.2325 \\
prim$\rightarrow$subj common  & 0.6707 & 0.843 & 0.7787 & 0.8965 \\
prim$\rightarrow$subj proper  & 0.6822 & 0.733 & 0.574 & 0.7412 \\
subj$\rightarrow$obj common  & 0.8954 & 0.9693 & 0.9554 & 0.9543 \\
subj$\rightarrow$obj proper  & 0.3419 & 0.3381 & 0.3407 & 0.4267 \\
unacc$\rightarrow$transitive  & 0.5095 & 0.4451 & 0.6149 & 0.6244
\end{tabular}
\end{table}
